# Supplementary material for: Processing Natural Language on Embedded Devices: How Well Do Transformer Models Perform?
Source: arXiv:2304.11520 source file (2024-03-07)
Supplement: Supplementary file 1 [file hs_appendix.tex]

\section{Robot Operating System (ROS)}
\label{robotOS}

We used Robot Operating System (ROS)~\cite{ros} (version 2) for controlling the robot and processing the input data.  
ROS-based architectures typically consist of two major components: \ci \textit{Node:} a process that performs computation and  \cb \textit{Topic:} communication channels used to transmit data between publishers and subscribers. 
%\cc \textit{Service:} this is equivalent to a client/server communication in a request/response pattern.
A ROS system consists of many small programs (nodes) which connect and continuously exchange messages. A single topic can have multiple publishers and subscribers. Nodes ``subscribe'' or ``publish'' to a topic. When multiple nodes access the same topic simultaneously, the requests are managed using first-in, first-out queues.

\begin{figure}[!htb]
\centering
% \vspace{-1.2em}
% \setlength{\abovecaptionskip}{-0pt}
    % \setlength{\belowcaptionskip}{-5pt}
    \hspace*{-2em}
\includegraphics[width=0.8\linewidth]{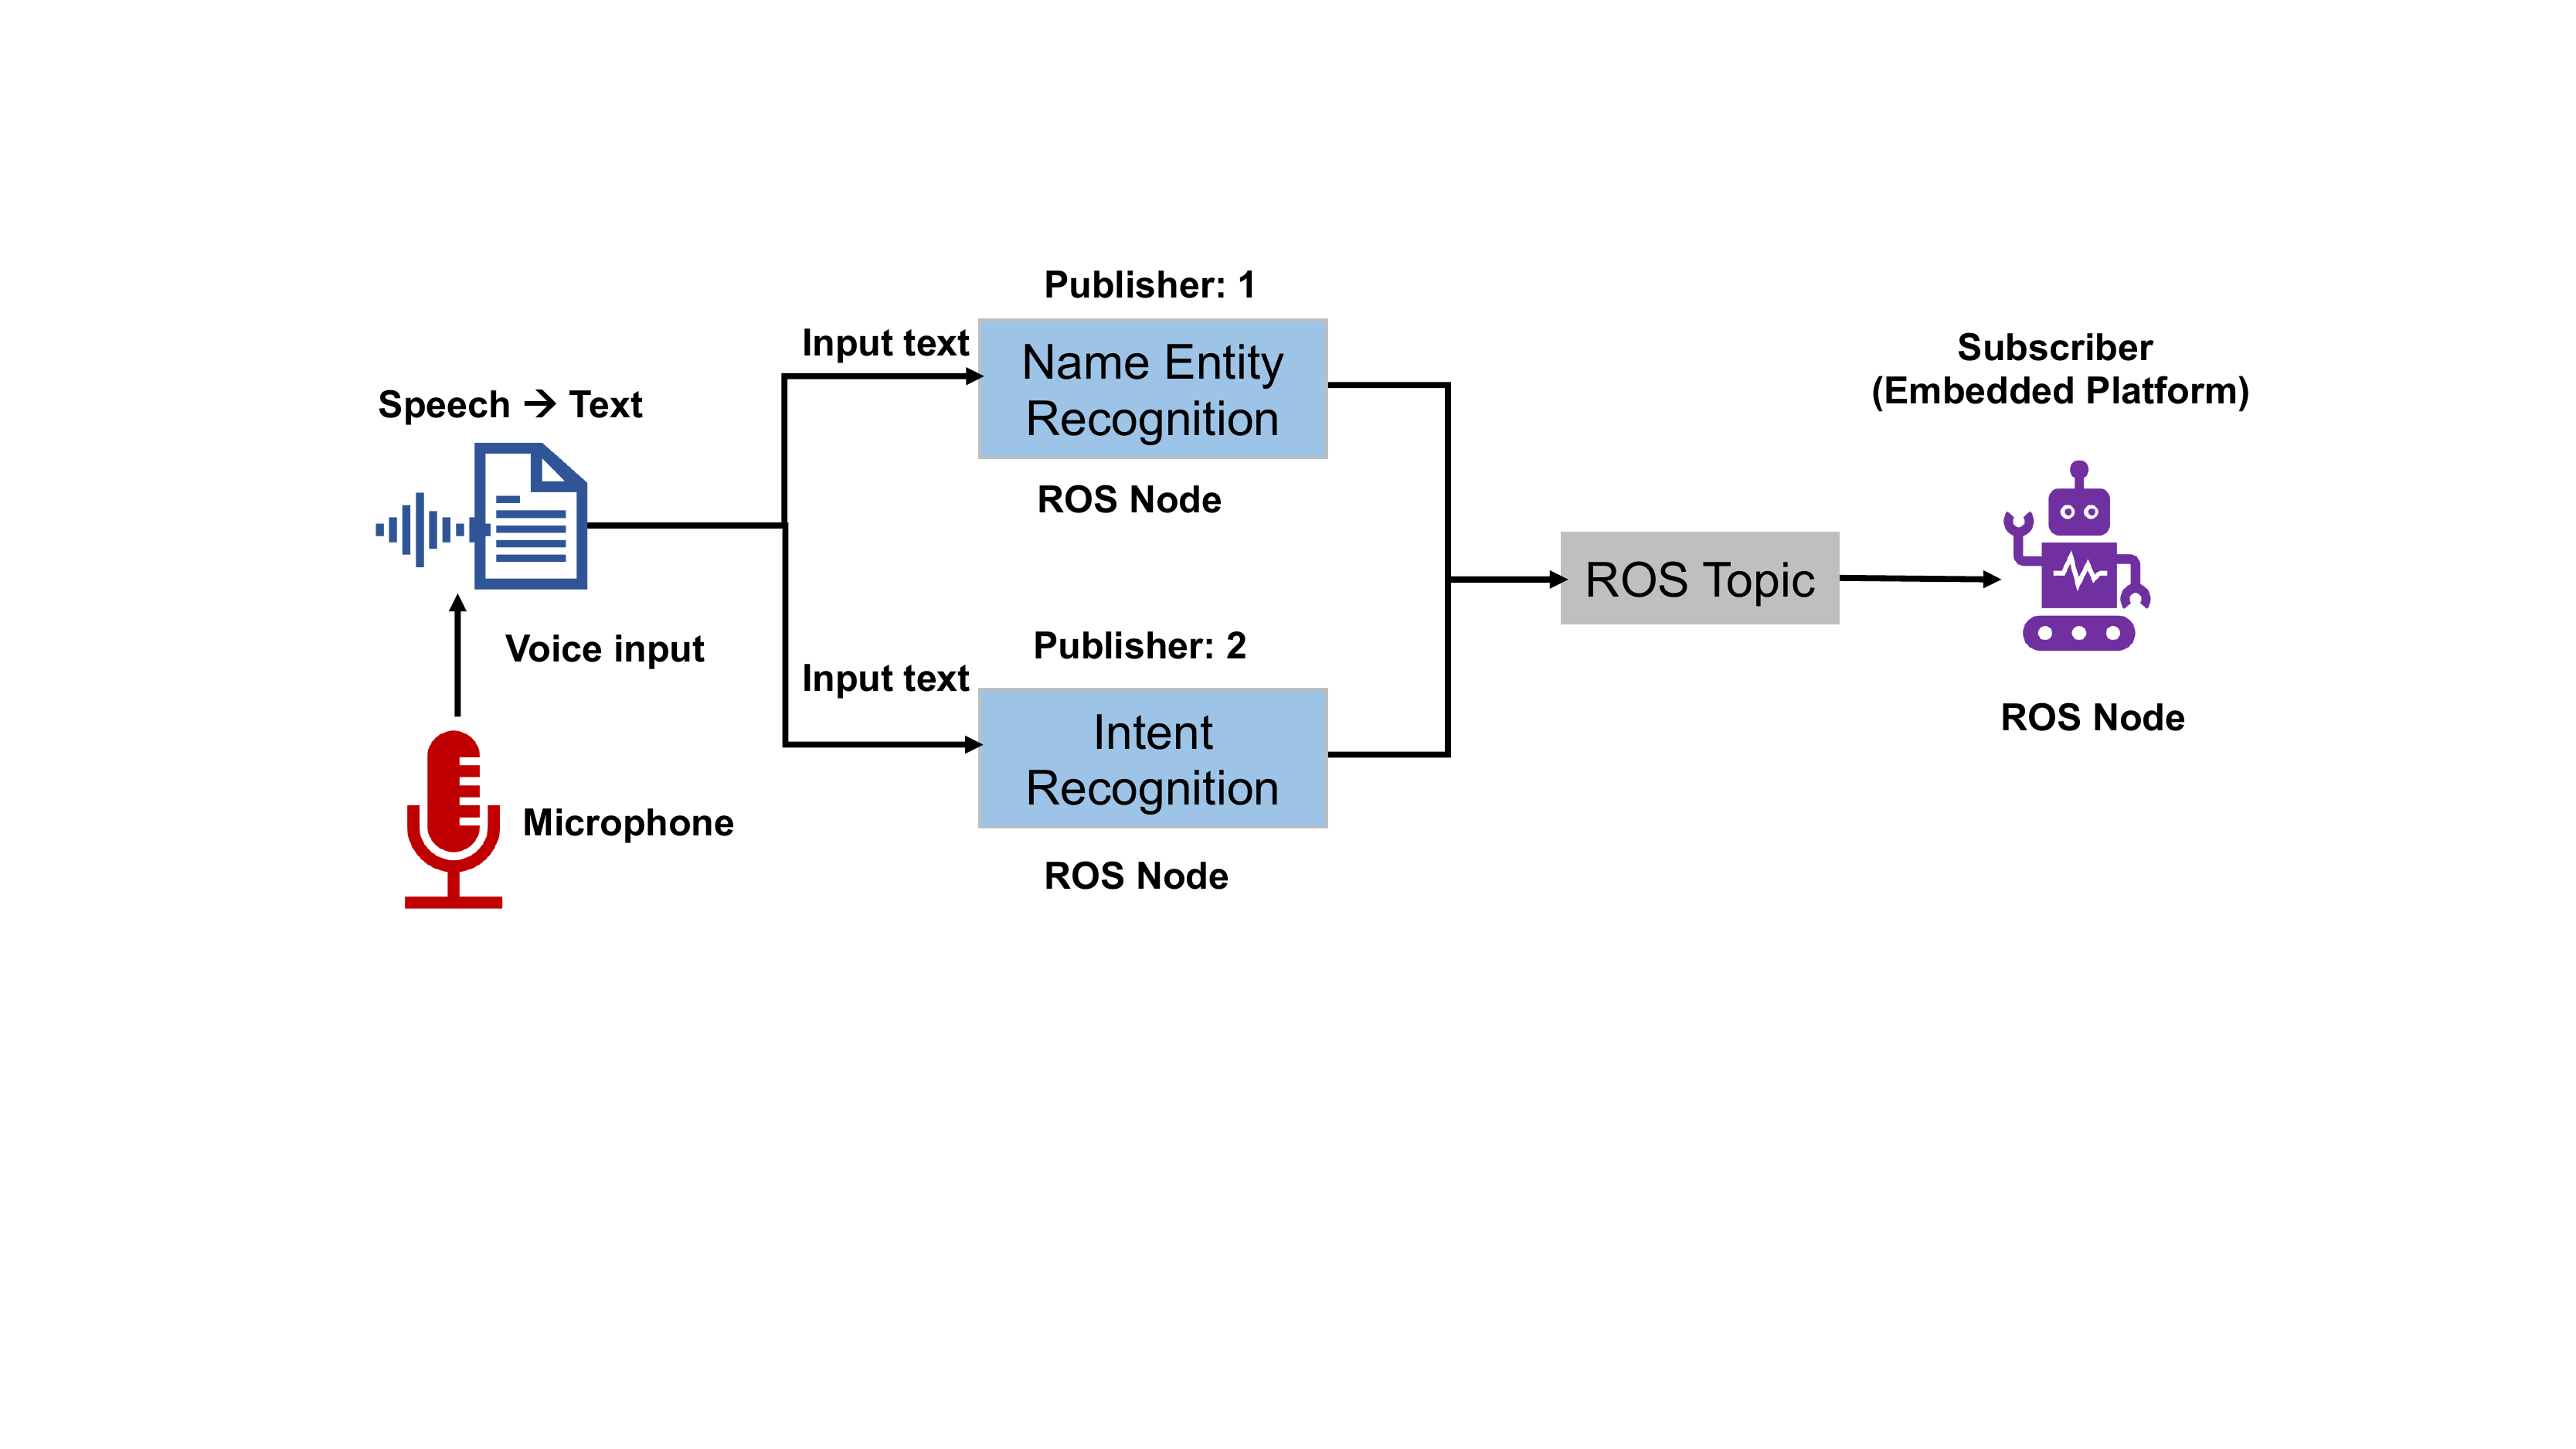}\vspace{-8mm}
\caption{Workflow of the ROS pub-sub model used in our experiments. %\noteby{MH}{FIX!}
}
\label{fig:pubsub}
\centering
\vspace{-3mm}
\end{figure}

We used standard ROS publisher-subscriber (pub-sub) models in our experiments. Figure~\ref{fig:pubsub} presents a high-level overview of our experiment setup. For example,~\enquote{Name Entity Recognition} and~\enquote{Intent Recognition} nodes send messages to the ROS topic~(\eg robot\_function). The~\enquote{Robot Driver} and nodes receive the messages from the corresponding topic and perform the task. 
